# Supplementary material for: Diverse Imitation Learning via Self-Organizing Generative Models
Source: arXiv:2205.03484 source file (2022-05-06)
Supplement: Supplementary file 1 [file robotics.tex]

\section{Further Experimental Results}
\subsection{Reaching Targets with a Robotic Arm}
Many robotic tasks require higher level planning \cite{yu2020meta}. In the context of reinforcement learning, high-level planning has been addressed under the umbrella of hierarchical reinforcement learning \cite{sutton1999between, frans2017meta}. We perform a set of  experiments using  \Cref{alg:sog-bc} for recovering higher-level modes in imitation of robotic tasks. We performed our experiment on FetchReach-v1 simulated robotic environment \cite{plappert2018multi}. This environment contains a 7-DoF robotic arm. The objective is to move the robotic arm such that its end point hits a desired target. We used a pretrained DDPG+HER \cite{lillicrap2015continuous, andrychowicz2017hindsight} model, as described in \cite{plappert2018multi}, to generate expert trajectories. We conducted two experiments. First, we selected three random targets and trained \Cref{alg:sog-bc} to imitate reaching those targets. Second, we spread the expert trajectories on a circle in the 3D space. In this latter experiment, when we used a one-dimensional latent variable, our method was able to imitate targets on only half of the circle (because of the angle warping in a circle). Therefore, we used an additional one-hot latent variable and performed search over both the continuous and discrete latent codes. In this manner, we were able to learn the entire circle. The results of the generated end points with the imitated policy are illustrated in \Cref{fig:fetch}. \Cref{alg:sog-gail} with $\lambda_S=1$ produced similar output, therefore we didn't present its results.

\begin{figure}[H]
    \centering
    \begin{subfigure}[t]{0.4\textwidth}
        \centering
        \includegraphics[height=2in]{sog-gail-clean/fig/fetch/fetch1.png}
        \caption{Three Targets}
    \end{subfigure}
    % \hspace{1in}
    \begin{subfigure}[t]{0.4\textwidth}
        \centering
        \includegraphics[height=2in]{sog-gail-clean/fig/fetch/fetch2.png}
        \caption{Reconstruction by SOG algorithm}
    \end{subfigure}
    \caption{\label{fig:fetch}\textbf{FetchReach.} Output samples of \Cref{alg:sog-bc} for FetchReach-v1 environment. \Cref{alg:sog-gail} produces similar results. Both plots are re-scaled such that possible choices of the targets fall within the unit cube. (a) Achieved targets upon imitation of three targets with a three-dimensional discrete latent code. Color coding corresponds to choices of the latent code. Gray lines help identify the 3D coordinates. Since the environment is fully deterministic, in order to get different trajectories, we injected a noise with a strength of 2\% of the maximum action magnitude on the actions. (b)  Achieved targets upon imitation of targets lying on a circle, using a combination of a 1-dimensional continuous code, and a two-dimensional one-hot code to choose between the two half-circles.}
\end{figure}
