# Supplementary material for: Diverse Imitation Learning via Self-Organizing Generative Models
Source: arXiv:2205.03484 source file (2022-05-06)
Supplement: Supplementary file 2 [file soft-assignment.tex]

% OUTLINE:
% 1. the generative model
% 2. the update rules
% 3. induction: assuming 1) and 2) (the winner conditions), if the modes were completely decoupled, then 1) and 2) holds and the winner defends championship
% 4. In practice the modes are coupled and due to the limited capacity (Lipschitzness) of the model, the winner mode for the boundary points might change

\section{Soft assignment EM algorithm} \label{appx:soft-assignment}
In this section, we provide a soft assignment batch EM solution to the problem of \cref{eq:gen-cluster} in \cref{sec:hard-assignment}. This approach relaxes the combinatorial problem by assuming the following probabilistic model:
\begin{align*}
p(\mY \given \mX ;\, \theta, \Pi) &= \prod_{i=1}^N p(\vy_{i} \given \vx_{i};\, \theta, \vpi_{i}) \\
p(\vy_{i} \given \vx_{i};\, \theta, \vpi_{i}) &= \sum_{k=1}^K p(\vy_{i} \given \vx_{i}, \vz_{i}=k;\,\theta) p(\vz_{i}=k ;\, \vpi_{i})\\
&=\sum_{k=1}^K p(\vy_{i} \given \vx_{i}, \vz_{i}=k;\,\theta) \pi_{ik}
\end{align*}
where the parameters of the model include $\theta$ and $\Pi$. That is, the model assumes a multi-mode likelihood parameterized by $\theta$ and data-point-specific cluster assignment probabilities $\Pi = \{\vpi_{1}, \dots, \vpi_{N}\}$ and $\vpi_{i} = \begin{bmatrix} \pi_{i1} & \cdots & \pi_{iK} \end{bmatrix}^T$.
% In this section, we provide a generalization to \cref{sec:hard-assignment} for the case where $\sigma$ is not assumed to be small. The optimization is done by alternating between the standard expectation step (E-step) and the maximization step (M-step).

With the iteration number denoted with superscript $(\cdot)^{(t)}$, the EM steps are the following:

\textbf{The E step}

For all $i=1,\ldots,N$, calculate:
\begin{align}
q_{i}^{(t)}(\vz) &= p(\vz_i \given \vx_i,\vy_i;\,\vpi^{(t)},\theta^{(t)})\nonumber\\
\text{\emph{i.e.} \quad}q_{i}^{(t)}(\vz = k) &= \frac{p(\vy_i \given \vx_i, \vz=k;\, \theta^{(t)}) \pi_{ik}^{(t)}}{\sum_{l=1}^K p(\vy_i \given \vx_i, \vz=l;\, \theta^{(t)}) \pi_{il}^{(t)}} \equiv r_{ik}^{(t)}\label{eq:soft-assmnt-e}
\end{align}
% where
% \begin{align*}
% r^{(t)}_{ik} &=p(\vy_{i}|\vz_{i}=k,\vx_{i}; \theta^{(t)})\\
% &= \frac{p(\vy_{i}|\vz_{i}=k,\vx_{i}; \theta^{(t)})\pi_{ik}}{\sum_{l=1}^K p(\vy_{i}|\vz_{i}=l,\vx_{i}; \theta^{(t)})\pi_{il}}
% \end{align*}

\textbf{The (Batch) M step}

Calculate
\begin{align}
\theta^{(t+1)}, \Pi^{(t+1)} &= \argmax_{\theta, \Pi} \Eoper_{\mZ\sim q^{(t+1)}}[\log P(\mY, \mZ \given \mX;\, \theta, \Pi)]\nonumber\\
&= \argmax_{\theta, \Pi} \sum_{i\in B} \sum_{k=1}^{K} r_{ik}^{(t)} \log \pi_{ik} + \sum_{i\in B} \sum_{k=1}^{K} r_{ik}^{(t)} \log p\left(\vy_i \;\left\vert\; \vx_i, \vz_i=k;\, \theta\right.\right)\label{eq:soft-assmnt-m}
\end{align}
where $B$ is the set of mini-batch data indices for the iteration.

Optimizing the first term in \cref{eq:soft-assmnt-m} for each $i$,
\[
\begin{array}{rl}
    \underset{\pi_{ik}}{\mathrm{maximize}} & \displaystyle\sum_k r_{ik}^{(t)} \log \pi_{ik} \\[1.5em]
    \text{s.t.} & \displaystyle\sum_{k=1}^K \pi_{ik} = 1
\end{array}
\]
gives the optimal solution for $\pi$ in the $t+1$ step  
\begin{equation}
\pi_{ik}^{(t+1)} =  \frac{r_{ik}^{(t)}}{\sum_{k=1}^K r_{ik}^{(t)}} = r_{ik}^{(t)} \label{eq:soft-assmnt-pi}
\end{equation}

Optimizing the second term in \cref{eq:soft-assmnt-m} results in (stochastic) gradient ascent updates of $\theta$:
\begin{equation}
\theta^{(t+1)} = \theta^{(t)} + \eta \sum_{i=1}^N \sum_{k=1}^K r_{ik}^{(t)} \nabla_{\theta} \log p\left(\vy_i \given \vx_i, \vz_i=k;\, \theta\right) \label{eq:soft-assmnt-theta}
\end{equation}
% $$\frac{\partial}{\partial \theta}  \sum_{i=1}^N\left[ r_{ik} \log\pi_{ik} - || f_\theta(\vz_{\kappa^{(i)}}, \vx_{i})- \vy_{i}||^2\right]$$

Based on the update rules of \cref{eq:soft-assmnt-e,eq:soft-assmnt-pi,eq:soft-assmnt-theta}, we are going to show that each of $\{\vpi_i\}_{i=1}^N$ will in practice converge to one-hot distributions.

To simplify the analysis, we first consider a batch size of 1. This doesn't affect the E-step much, because the update of each $\vpi_i$ is independent. However in the M-step, $\theta$ is optimized for only one data point $(\vx_i, \vy_i)$.

Assuming \cref{eq:k-win-1,eq:k-win-2}, i.e., the $\kappa$\textsuperscript{th} code ``wins'' among the $K$ latent codes in the $t$\textsuperscript{th} step, we are going to show that the $\kappa$\textsuperscript{th} code is likely to ``defend its championship'' after one iteration of EM optimizaiton.
% \begin{tcolorbox}
\begin{align}
& p(\vy_i \given \vx_i, \vz=\kappa;\,\theta^{(t)}) > p(\vy_i \given \vx_i, \vz=l;\,\theta^{(t)}), \quad \forall l \neq \kappa \label{eq:k-win-2}\\
& \pi_{i\kappa}^{(t)} > \pi_{il}^{(t)},\quad \forall l \neq \kappa \label{eq:k-win-1}
\end{align}
% \end{tcolorbox}
Consider the gradient ascent update in \cref{eq:soft-assmnt-theta}, which becomes
\[\eta \sum_{k=1}^{K} r_{ik}^{(t)} \nabla_{\theta} \log p\left(\vy_i \given \vx_i, \vz_i=k;\, \theta\right).\]
Because of \cref{eq:k-win-1,eq:k-win-2}, \[r_{i\kappa}^{(t)} > r_{il}^{(t)},\quad \forall l \neq \kappa,\] therefore $\kappa$\textsuperscript{th} gradient, $\nabla_{\theta} \log p\left(\vy_i \given \vx_i, \vz_i=\kappa;\, \theta\right)$ dominates, and the model is improved more for the $\kappa$\textsuperscript{th} mode. Arguably, this leads to
\begin{align*}
\frac{p\left(\vy_i \given \vx_i, \vz_i=\kappa;\, \theta^{(t+1)}\right)}{p\left(\vy_i \given \vx_i, \vz_i=\kappa;\, \theta^{(t)}\right)}
&\geq
\frac{p\left(\vy_i \given \vx_i, \vz_i=l;\, \theta^{(t+1)}\right)}{p\left(\vy_i \given \vx_i, \vz_i=l;\, \theta^{(t)}\right)},  &\forall l \neq \kappa &
\text{,\quad or}\\
\frac{p\left(\vy_i \given \vx_i, \vz_i=\kappa;\, \theta^{(t+1)}\right)}{p\left(\vy_i \given \vx_i, \vz_i=l;\, \theta^{(t+1)}\right)}
&\geq
\frac{p\left(\vy_i \given \vx_i, \vz_i=\kappa;\, \theta^{(t)}\right)}{p\left(\vy_i \given \vx_i, \vz_i=l;\, \theta^{(t)}\right)},  &\forall l \neq \kappa & \stepcounter{equation}\tag{\theequation}\label{eq:soft-assmnt-likelihood-ratio}
\end{align*}
If the \cref{eq:soft-assmnt-likelihood-ratio} above holds, \cref{eq:k-win-2} remains to hold after this iteration of update.

Now notice that combining \cref{eq:soft-assmnt-e,eq:soft-assmnt-pi}, we have a recursive relation
\[
\frac{\pi_{i\kappa}^{(t+1)}}{\pi_{il}^{(t+1)}} = \frac{r_{i\kappa}^{(t)}}{r_{il}^{(t)}} = \frac{\pi_{i\kappa}^{(t)}}{\pi_{il}^{(t)}} \frac{p\left(\vy_i \given \vx_i, \vz_i=\kappa;\, \theta^{(t)}\right)}{p\left(\vy_i \given \vx_i, \vz_i=l;\, \theta^{(t)}\right)}
\]
which together with \cref{eq:k-win-1,eq:k-win-2}, guarantees that $\dfrac{\pi_{i\kappa}^{(t+1)}}{\pi_{il}^{(t+1)}}$ increases compared to the $t$\textsuperscript{th} step and therefore \cref{eq:k-win-1} remains to hold after this iteration of update, too.

The ``proof'' above doesn't necessarily hold, because \cref{eq:soft-assmnt-likelihood-ratio} is not guaranteed after a gradient ascent step. It especially meet difficulties when 

and it showed the tendency of evolving from soft probabilities of $r_{ik}$ over $K$ modes to preference over one given mode for each data point, i.e the assigned probability gradually concentrates. 

self boosting ratio: 
\[\frac{\pi_{ik}^{(t+1)}}{\pi_{ij}^{(t+1)}} = \frac{r_{ik}^{(t)}}{r_{ij}^{(t)}} =  \frac{\pi_{ik}^{(t)}}{\pi_{ij}^{(t)}}\frac{p(y_i \given z_i=k, x_i, \theta^{(t)})}{p(y_i \given z_i=j,x_i,  \theta^{(t)})}\]
