# Supplementary material for: Diverse Imitation Learning via Self-Organizing Generative Models
Source: arXiv:2205.03484 source file (2022-05-06)
Supplement: Supplementary file 3 [file soft-em-intuition.tex]

\subsection{Soft Assignment EM} \label{sec:soft-em}
 First we observe  that if the dataset has distinct modes, then 
 %the intuition behind the observation that 
 the posterior distribution in the EM approach always tends to one-hot.
For simplicity, let us assume that the modes in dataset are \textcolor{blue}{balanced} and have the same number of data points. \textcolor{blue}{This leads to uniform cluster prior distribution at convergence: $\pi_k^t \rightarrow 1/K, k=1,\ldots, K$. } The posterior assignment distribution of a data point over the $K$ clusters (\Cref{eq:em-post}) is then simply proportional to the conditional likelihood for the  clusters, i.e.
\begin{subequations}
\begin{align}
r_{ik}^{t} &= p(z=k \given \vx_i, \vy_i;\: \boldsymbol\theta^{t}, \boldsymbol\Pi^{t}) \\&= \frac{p(\vy_i | \vx_i,z=k;\: \boldsymbol\theta^{t})\:\pi_k^t}{\sum_{l=1}^K p(\vy_i | \vx_i, z=l; \:\boldsymbol\theta^{t})\: \pi_l^t} \\&\approx \frac{p(\vy_i | \vx_i,z=k;\: \boldsymbol\theta^{t})}{\sum_{l=1}^K p(\vy_i | \vx_i, z=l; \:\boldsymbol\theta^{t})} 
\end{align}
\end{subequations}

Consider a specific data point $(\vx_i, \vy_i)$. Along the training using EM algorithm, at some step $t$, one of the cluster, $\kappa$, will have higher likelihood compared to the alternatives (because the likelihood conditioned on different clusters remaining perfectly equal is very unlikely), i.e. 
\begin{equation}
    p(\vy_i \given \vx_i, z=\kappa; \theta^{t}) > p(\vy_i \given \vx_i, z=l; \theta^{t}), \quad \text{if } l \neq \kappa.
    \label{eq:em-kappa-winning}
\end{equation}
This leads to a higher posterior for this ``winning'' cluster compared to its alternatives:
\[r^t_{i\kappa} > r^t_{il}, \quad \text{if } l \neq \kappa,\]
Therefore, due to the M step, the ``winning'' cluster gains more weight in the loss function, and tends to be improved more than the alternatives, so that \Cref{eq:em-kappa-winning} remains to hold, and the ``winning margin'', $\dfrac{p(\vy_i \given \vx_i, z=\kappa)}{p(\vy_i \given \vx_i, z=l)}$, even increases.

As the result of such positive feedback, the posterior distribution tends to one-hot and $r^t_{i\kappa} \approx 1$, while $r^t_{il} \approx 0$ for $l \neq \kappa$.

Now we show that this EM posterior can not be exactly one-hot and will always have a finite gap when the likelihood function is assumed to be Gaussian, i.e. $p(\vy_i \given \vx_i, z) = \mathcal{N}(\vy; f_\theta(z, \vx), \sigma^2 \mI)$, and the gap is a function of $\sigma$. Because the Gaussian distribution is non-zero in the whole domain, and the prediction function $f_\theta$ has finite output, the posterior for the non-dominating clusters is always finite, i.e. $r^t_{il} > 0$ is finite, even for $l \neq \kappa$. This has two consequences:

\begin{enumerate}
    \item The non-dominating clusters will have non-negligible contribution to the loss (unlike in the case of  SOG where the search is done over one-hot codes). The loss of EM algorithm (we focus on the M-step, because it has direct correspondence to the loss of SOG) for a data point $(\vx_i, \vy_i)$ is given by the expected negative log probability \[\mathcal{L}(\theta) = -\sum_l r^t_{il} \log p(\vy_i \given \vx_i, z=l \;;\; \theta).\] Now that the $r^t_{il}$ is not one-hot, $\log p(\vy_i \given \vx_i, z=l \;;\; \theta)$ will have contribution to the loss for $l\neq \kappa$, making it larger than the loss attained by SOG, where $r^t_{il} = 0$ for $l \neq \kappa$. This is confirmed by the plot \Cref{fig:em-toy-rebuttal:onehot} in where the loss of EM drops significantly when calculated after converting the posterior to exactly one-hot like in SOG.
    
    \item As a consequence, the contribution to the loss from the non-dominating clusters will keep the convergence point slightly away from the optimal solution that maximizes the dominating conditional likelihood $p(\vy_i \given \vx_i, z=\kappa \;;\; \theta)$.
\end{enumerate}

\textcolor{blue}{\subsubsection*{Experiment setup}}
In this section, we illustrate some of  the points we have made above regarding soft and hard variants of EM, using a toy experiment. This experiment demonstrates that both variants are able to recover the structure (three modes) in the dataset and illustrate the effectiveness of \Cref{alg:sog}. We use a multi-modal linear generative model to generate the dataset of tuples $\{(\vx_i, \vy_i, z_i)\}_{i = 1}^N$. Concretely, $\vx_i \sim \mathcal{N}(0, \mI_2), \vy_i = \vx_i + \vw_{z_i} + \bm{\epsilon_i}$, where $z_i \sim \mathrm{Categorical}(\frac{1}{3},\frac{1}{3},\frac{1}{3})$, $\bm{\epsilon}_i \sim \mathcal{N}(0,0.01^2 \mI_2)$. That is, $\vx_i \in \mathbb{R}^2$ is drawn from a unit Gaussian distribution, and $\vy_i \in \mathbb{R}^2$ is computed by offsetting $\vx_i$ by amount of $\vw_{z_i} \in \mathbb{R}^2$ according to its corresponding mode $z_i \in \{1, 2, 3\}$.

In both the EM and SOG we train a linear model $f_{\boldsymbol\theta}(z, \vx) = \boldsymbol\theta \begin{bmatrix} \texttt{one\_hot}(z) \\ \vx \end{bmatrix}$, parameterized by $\boldsymbol\theta \in \mathbb{R}^{5\times 2}$ on the data such that the marginal likelihood is maximized.

\subsubsection*{Results}
The experiments on the toy example showed that both variants are able to produce satisfactory fitting results. As we can see in \Cref{fig:em-toy}, both EM and SOG recover the structure (three modes) existing in the ground truth $\mY$ (colors are randomly assigned to distinguish different modes). Furthermore, as expected, the soft variant ultimately leads to one-hot posterior distribution among latent codes in the discrete code case, which is assumed by SOG. \Cref{fig:em-toy-code} shows the posterior distribution 
%(where the color coding is based on the ground truth modes)
from EM algorithm gradually converges from almost uniform distribution in epoch 2 to one-hot in epoch 100 when its loss converges, which justifies SOG's way of approximation to the posterior. Although there are no significant visual distinctions among the synthesized samples in \Cref{fig:em-toy}, we comment that SOG is more reliable to attain good performance in terms of loss value and convergence speed compared to EM algorithm. Below we provide a detailed analysis.

%%%%%%%%%%%%%%%%%%%%%%%%%% REVISION %%%%%%%%%%%%%%%%%%%%%%%%%%
% Now we further investigate the convergence and final performance of SOG and EM algorithm as shown in \Cref{fig:em-toy-loss}. 
In \Cref{fig:em-toy-rebuttal:original}, the training curves of the two algorithms are plotted in both linear and logarithm scale, and they show that SOG not only has a faster convergence speed, but also a lower loss at convergence, despite the fact that the posterior distribution of the EM algorithm goes to one-hot just like the hard-assignment used by SOG (shown in \Cref{fig:em-toy-code}). This raises the question: now that EM behaves like SOG asymptotically, why does it have inferior performance? The reason is that, limited by the Gaussian likelihood assumption (which is boundless), the EM approach can never attain purely one-hot posterior, which is shown as follows. In particular, the EM approach maximizes the expected likelihood of the data (where expectation is taken over all the latent codes), whereas the SOG maximizes the likelihood of the data conditioned at the code where it is maximum.  Both of the consequences can be alleviated by decreasing the standard deviation $\sigma$ assumed in the Gaussian likelihood. Indeed, when we decrease $\sigma$ by two orders of magnitude from its original value $1$ to $0.01$, the training curve of EM and SOG match as shown in \Cref{fig:em-toy-rebuttal:low-sigma}.

% Compared to the EM approach, SOG is free from the hyperparameter tuning for $\sigma$, and more reliably yields
% This means that $\sigma$ can be used to control the balance between mode specialization and generalization.

%%%%%%%%%%%%%%%%%%%%%%% END OF REVISION %%%%%%%%%%%%%%%%%%%%%%%

\begin{figure}
    \centering
    \begin{subfigure}[t]{0.32\textwidth}
        \centering
        \includegraphics[width=\hsize]{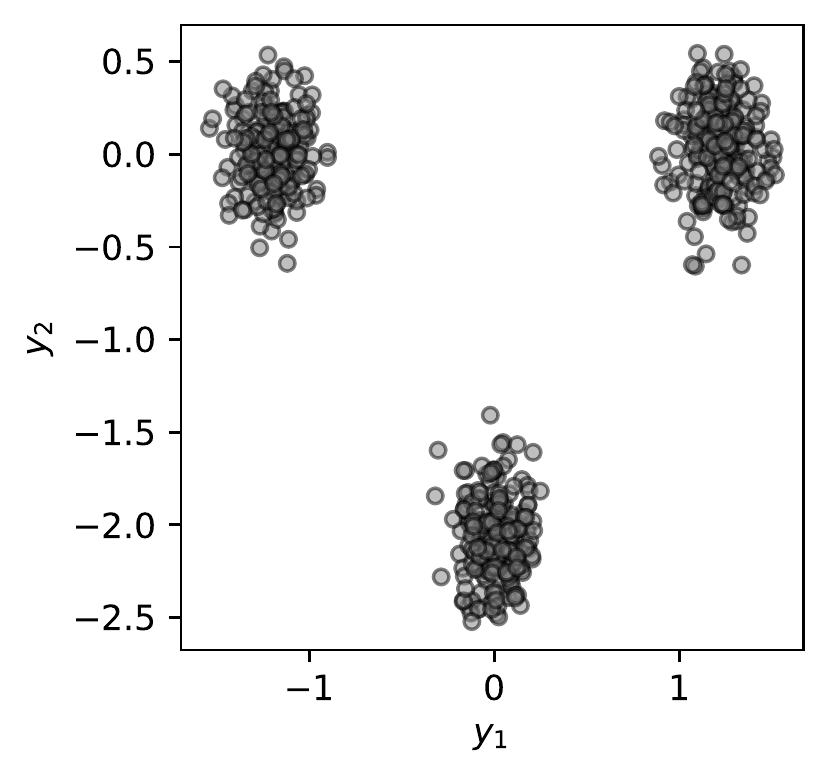}
        \caption{The ground truth $\mY$}
    \end{subfigure}
    \begin{subfigure}[t]{0.32\textwidth}
        \centering
        \includegraphics[width=\hsize]{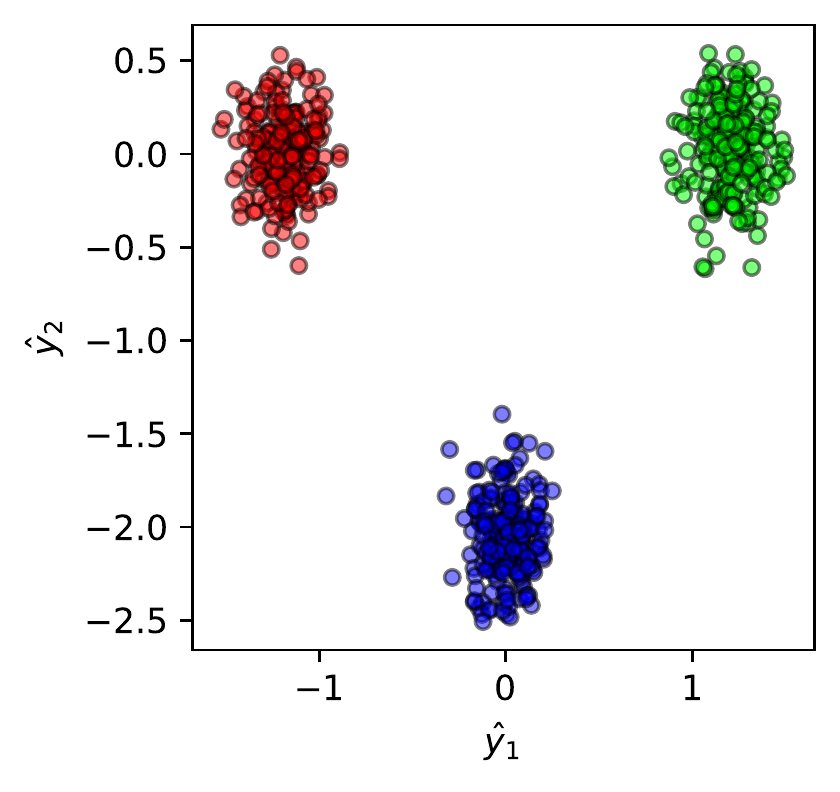}
        \caption{The EM predictions}
    \end{subfigure}
    \begin{subfigure}[t]{0.32\textwidth}
        \centering
        \includegraphics[width=\hsize]{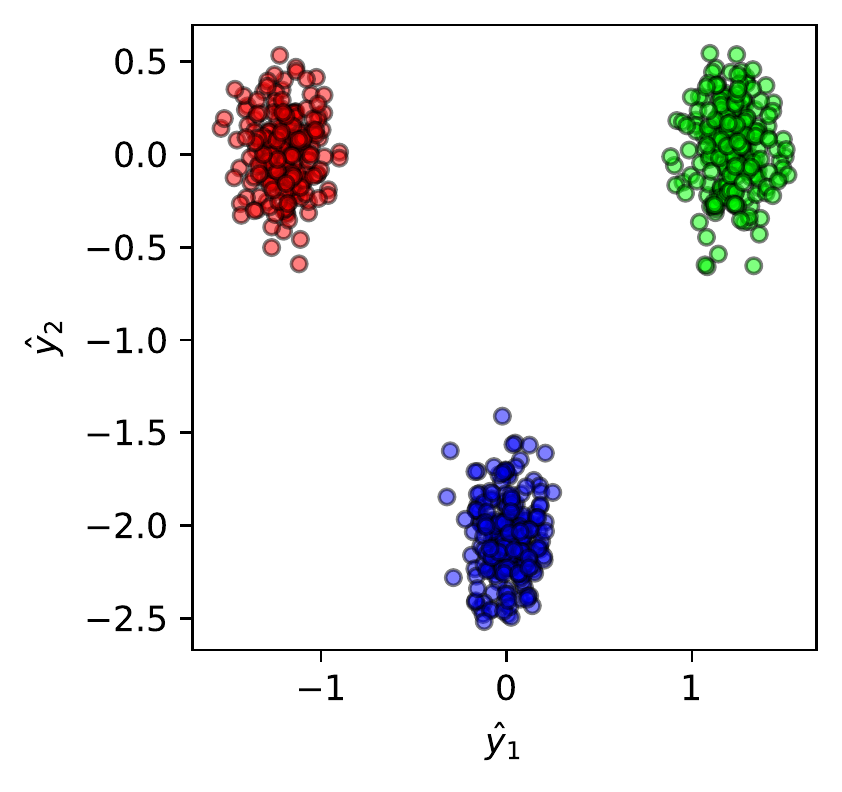}
        \caption{The SOG predictions}
    \end{subfigure}
    \caption{\label{fig:em-toy}\textbf{Three-mode clustering toy example.} Ground truth and model predictions at convergence. Points are colored-coded with the  latent code assignments from the EM algorithm.}
\end{figure}

\begin{figure}
    \centering
    \includegraphics[width=0.7\hsize]{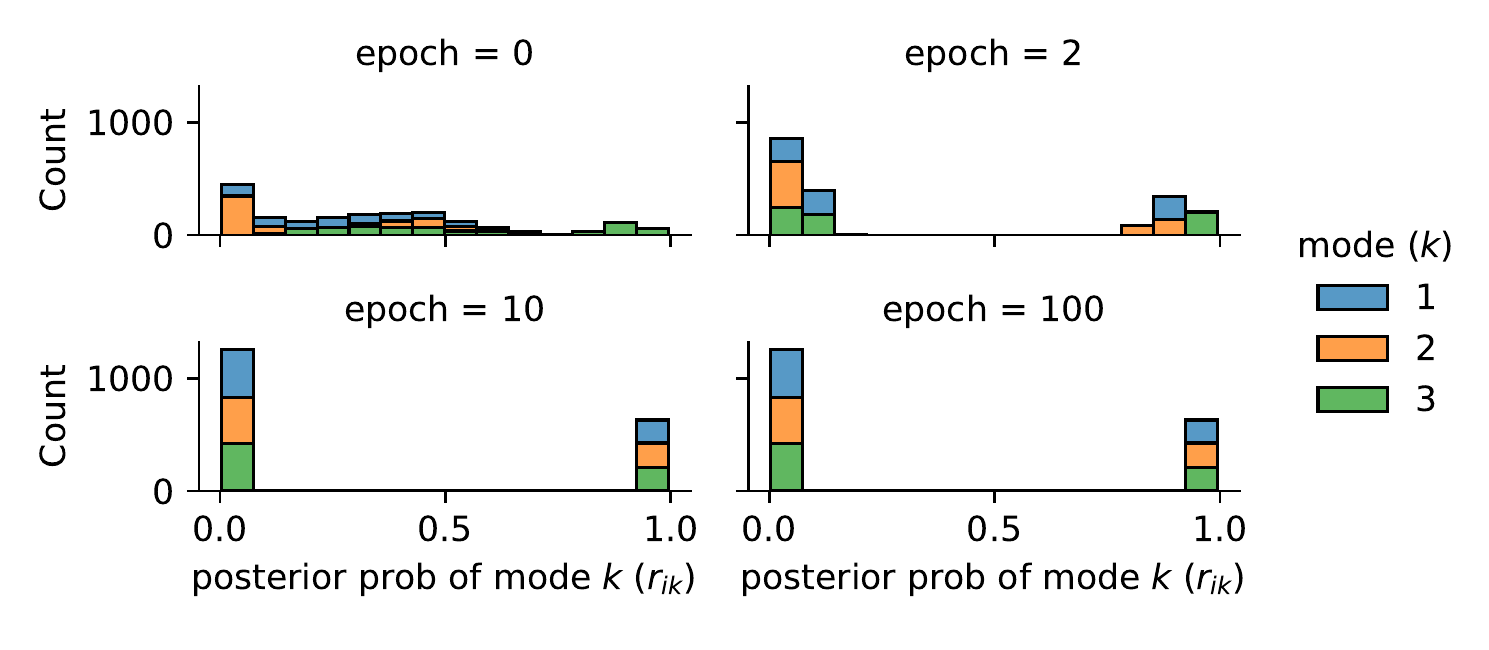}
    \caption{\label{fig:em-toy-code}Posterior distribution of soft EM along training}
\end{figure}

\begin{figure}
    \centering
    \begin{subfigure}[t]{0.32\textwidth}
        \centering
        \includegraphics[width=\hsize]{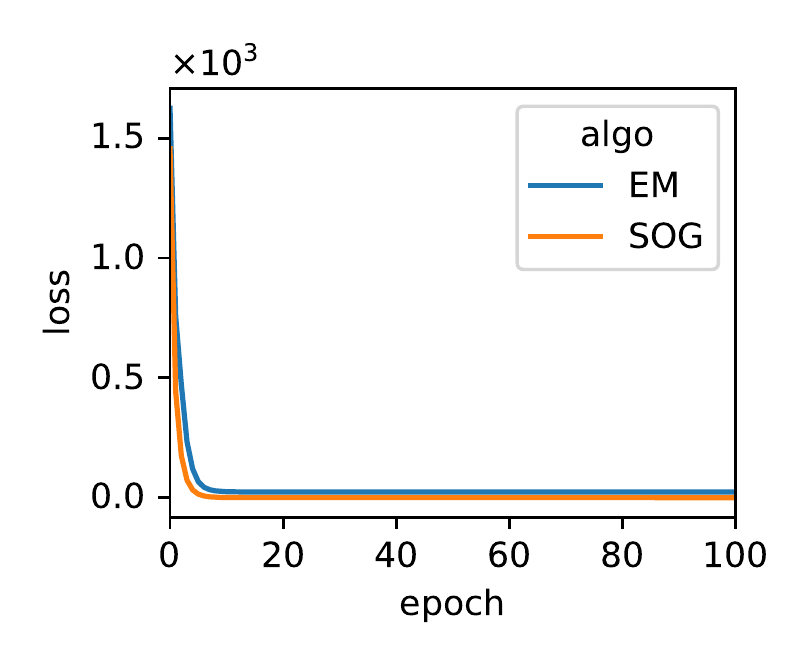}
        \includegraphics[width=\hsize]{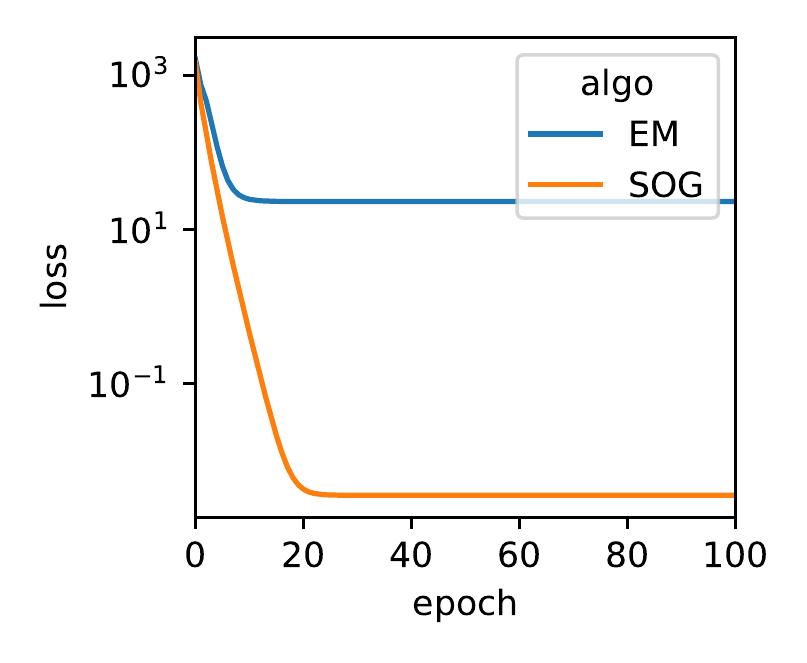}
        \caption{\label{fig:em-toy-rebuttal:original}$\sigma = 1$ for EM. Upper: linear-scale; lower: log-scale}
    \end{subfigure}
    % \hspace{1in}
    \hfill
    \begin{subfigure}[t]{0.32\textwidth}
        \centering
        \includegraphics[width=\hsize]{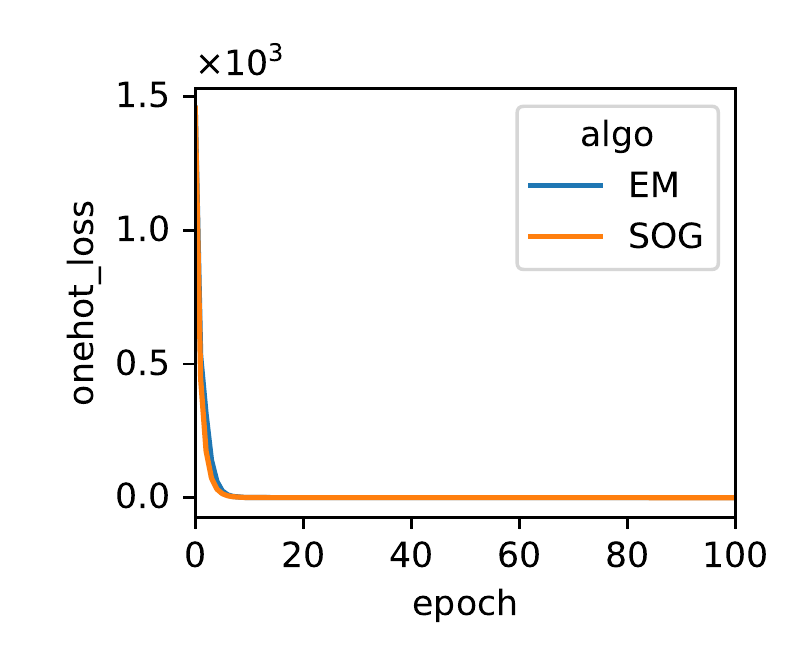}
        \includegraphics[width=\hsize]{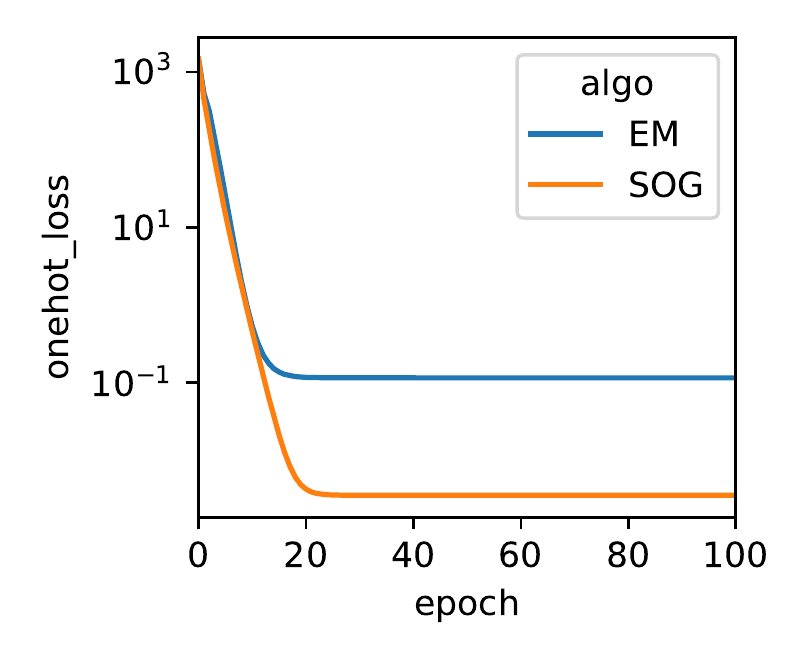}
        \caption{\label{fig:em-toy-rebuttal:onehot}$\sigma = 1$ for EM. Posterior is converted to one-hot when calculating the loss for plotting. Upper: linear-scale; lower: log-scale}
    \end{subfigure}
    \hfill
    \begin{subfigure}[t]{0.32\textwidth}
        \centering
        \includegraphics[width=\hsize]{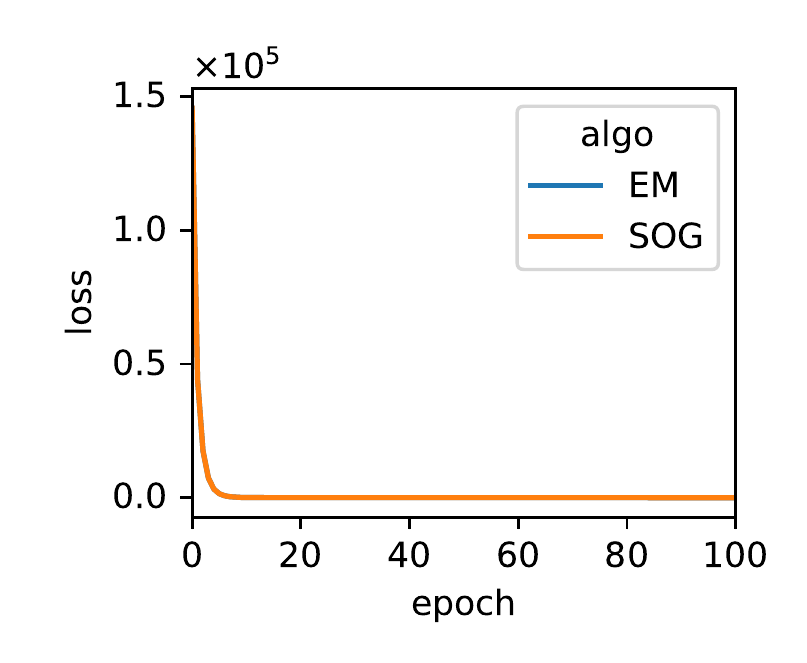}
        \includegraphics[width=\hsize]{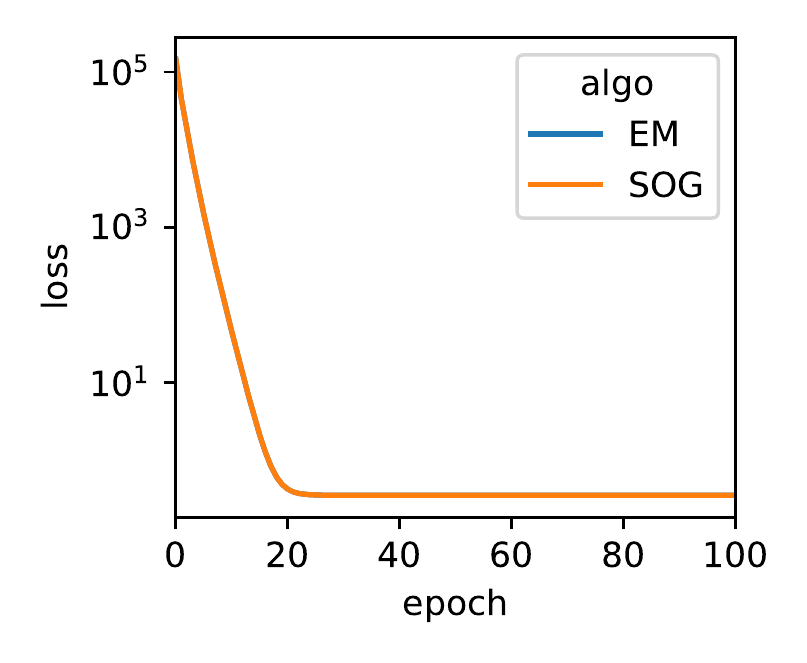}
        \caption{\label{fig:em-toy-rebuttal:low-sigma}$\sigma = 0.01$ for EM. Upper: linear-scale; lower: log-scale}
    \end{subfigure}
    \caption{\label{fig:em-toy-loss} The training curve of the EM algorithm vs that of SOG.}
\end{figure}
% \begin{figure}

%     \centering
%     \includegraphics[width=0.49\hsize]{fig/em-toy/em_toy_loss_curve.pdf}
%     \includegraphics[width=0.49\hsize]{fig/em-toy/em_toy_loss_curve_log.pdf}
%     \caption{\label{fig:em-toy-loss}The training curve of the EM algorithm vs that of SOG. The loss is the expected negative log-likelihood used in the M step.}
% \end{figure}

\iffalse 
A soft version of the EM algorithm to efficiently solve Eq.(~\ref{eq:cluster-opt}) is given in the appendix. We show how for each $i$, $r_{il}$'s converge to one-hot codes, where only one of the entries becomes 1 and rest converge to $0$,\fi

% Lastly, we shall note that it can be verified that the update rule for prior probabilities in \Cref{eq:prior-update} becomes:
% \begin{equation}
% \label{eq:opt_pi}
%     \pi_k^{t+1} = \frac{N_k}{N},
% \end{equation}
% where $N_k=\sum_{i=1}^{N}\mathbf{1}(\kappa^{(i)}=k)$, that is the number of data points for which the $k$'th code is the best. However, since \Cref{eq:sog-mstep} can be calculated irrespective of the values of $\pi_k$'s, \Cref{eq:opt_pi} is skipped in \Cref{alg:sog}.
