# Supplementary material for: Diverse Imitation Learning via Self-Organizing Generative Models
Source: arXiv:2205.03484 source file (2022-05-06)
Supplement: Supplementary file 4 [file sog-results.tex]

\section{SOG Results on Toy Data} \label{appx:sog-results}
In this section we briefly demonstrate success of SOG algorithm in distribution learning.
