# Supplementary material for: Diverse Imitation Learning via Self-Organizing Generative Models
Source: arXiv:2205.03484 source file (2022-05-06)
Supplement: Supplementary file 5 [file continuous-old.tex]

In this section, we analyse the behavior of the data log likelihood when SOG is applied for the continuous latent variables case. 
%relationship between optimization procedure of \Cref{alg:sog}, and \Cref{eq:max-marginal-likelihood} for continuous latent variables. 
Consider the following identity \citep{chib1995marginal}, a direct result of the Bayes' rule:
\begin{equation} \label{eq:BMI}
\resizebox{.89\linewidth}{!}{$
    \underbrace{\log p(\vy | \vx; \boldsymbol\theta)}_{\substack{\text{data} \\\text{log-likelihood}}} =
    \underbrace{\log p(\vy | \vz, \vx; \boldsymbol\theta)}_\text{SOG objective} - \underbrace{\log \frac{p(\vz | \vx,\vy;\boldsymbol\theta)}{p(\vz)}}_\text{gap}; \ \forall \vz.$}
\end{equation}
This identity describes a gap between the objectives in SOG and the data log-likelihood. The rest of this section aims to show that under certain reasonable assumptions about the posterior distributions of the latent codes, the SOG algorithm increases the overall data log-likelihood function and reaches a maximum, before it starts overfitting, when the posterior distributions become too narrow. We also show that such overfitting can be avoided, and the data log-likelihood be kept high by using a limited number of latent code samples over which the minimum loss is calculated in the first step of SOG. 

\Cref{alg:sog} searches for a latent code $\vz^*$ that maximizes the SOG term above. In \Cref{eq:BMI}, the marginal data log-likelihood term is not a function of the latent variable. Therefore,
\begin{subequations}
\begin{align}
    \vz^* &= \argmax_{\vz}\, \log p(\vy | \vz, \vx; \boldsymbol\theta) \\ 
    &= \argmax_{\vz} \,\log \frac{p(\vz | \vx,\vy; \boldsymbol\theta)}{p(\vz)}. \label{eq:argmax-gap}
\end{align}
\end{subequations}
We assume the model to be realized with a high-capacity neural network. Hence, we can assume an arbitrary form for the posterior distribution in \Cref{eq:argmax-gap}, e.g. a Gaussian \citep{kingma2013auto}:
\begin{equation}
    p(\vz | \vx,\vy; \boldsymbol\theta) = \mathcal{N} (\vz;\boldsymbol\mu_{\boldsymbol\theta}(\vx, \vy), \boldsymbol\Sigma_{\boldsymbol\theta}(\vx, \vy)).
\end{equation}
For a Gaussian form of the prior and the posterior, the gap in \Cref{eq:argmax-gap} can be written in closed form:
\begin{subequations}
\begin{alignat}{2} \label{eq:z-star}
    \begin{split}
    \vz^* =& \argmax_\vz -\frac{1}{2}\left[(\vz-\boldsymbol\mu)^T\boldsymbol{\Sigma}^{-1}(\vz-\boldsymbol\mu)^T\right]\\
    &-\frac{1}{2}\log\det\boldsymbol\Sigma+\frac{1}{2}\vz^T\vz
    \end{split}\\
    =&\label{eq:z-star-result}\begin{cases}
    (\mI-\boldsymbol\Sigma)^{-1}\boldsymbol\mu, & \text{if } \mI-\boldsymbol\Sigma \succ \boldsymbol0\\
    \text{unbounded},              
    & \text{otherwise}
    \end{cases}
\end{alignat}
\end{subequations}
where $\boldsymbol\mu$ and $\boldsymbol\Sigma$ denote a shorthand for $\boldsymbol\mu_{\boldsymbol\theta}(\vx, \vy)$ and $\boldsymbol\Sigma_{\boldsymbol\theta}(\vx, \vy)$. Since the model is trained to create mutual information between the data points and latent codes, \textcolor{blue}{the posterior distribution develops more certainty than the prior, that is $\mI\succ\boldsymbol\Sigma$}. Hence, \Cref{eq:z-star-result} yields $\vz^*=(\mI-\boldsymbol\Sigma)^{-1}\boldsymbol\mu$.
Next, we use the $\vz^*$ derived above to obtain the gap term in closed form:
\begin{subequations} \label{eq:gap-all}
\begin{alignts}
    g(\boldsymbol\mu, \boldsymbol\Sigma)\equiv&\max_{\vz} \, \log \frac{p(\vz | \vx,\vy; \boldsymbol\theta)}{p(\vz)}\\
    \begin{split}
    =&-\frac{1}{2}\left[(\vz-\boldsymbol\mu)^T\boldsymbol{\Sigma}^{-1}(\vz-\boldsymbol\mu)^T\right]\:\Bigr|_{\vz=\vz^*} \; \\&\,-\frac{1}{2}\log\det\boldsymbol\Sigma
    \end{split}\\
    \begin{split}
    =&-\frac{1}{2}\left[(\vz-\boldsymbol\mu)^T\boldsymbol{\Sigma}^{-1}(\vz-\boldsymbol\mu)^T\right]\:\Bigr|_{\vz=\vz^*} \;\\&\, -\frac{1}{2}\log\det\boldsymbol\Sigma
    \end{split}\\
    \begin{split}
    =&\frac{1}{2}(\mQ^T\boldsymbol\mu)^T(\mI-\boldsymbol\Lambda)^{-1}(\mQ^T\boldsymbol\mu)\\&\,-\frac{1}{2}\log\det\boldsymbol\Sigma 
    \end{split}\label{eq:lambda}\\
    =&\frac{1}{2}\boldsymbol\mu^T\left(\mQ(\mI-\boldsymbol\Lambda)\mQ^T\right)^{-1}\boldsymbol\mu-\frac{1}{2}\log\det\boldsymbol\Sigma\\
    =&\frac{1}{2}\boldsymbol\mu^T(\mI-\boldsymbol\Sigma)^{-1}\boldsymbol\mu-\frac{1}{2}\log\det\boldsymbol\Sigma \\
    \leq& \|\boldsymbol\mu\|^2 \sqrt{\Tr((\mI-\boldsymbol\Sigma)^{-2})}-\frac{1}{2}\log\det\boldsymbol\Sigma \label{eq:gap}\\
    =& \|\boldsymbol\mu\|^2 \sqrt{\Tr((\mI-\boldsymbol\Lambda)^{-2})}-\frac{1}{2}\log\det\boldsymbol\Lambda \label{eq:gap-diag}\\
    \equiv& h(\vmu, \mLambda)\label{eq:gap-h}, 
\end{alignts}
\end{subequations}
where in \Cref{eq:lambda,eq:gap-diag}, the covariance matrix is diagonalized as $\boldsymbol\Sigma=\mQ\boldsymbol\Lambda\mQ^T$. Also, \Cref{eq:gap} follows from the fact that $\forall\mA,\mB\succeq\boldsymbol0;\,\Tr(\mA\mB) \leq \sqrt{\Tr(\mA^2)\Tr(\mB^2)}$.

% Next we note that as the SOG loss decreases, the posterior distribution becomes narrower and ....
Now we more closely study the properties of the gap upper bound $h(\vmu, \mLambda)$, and show that the gap is not large under the following assumptions and arguments:
\begin{enumerate}
    \item Since \Cref{alg:sog} optimizes its objective for latent codes sampled from a Gaussian prior distribution, $\boldsymbol\mu$ remains bounded.

    \item \textcolor{gray}{Along the initial training phase of the model, the SOG objective increases and the gap term in \Cref{eq:BMI} decreases, leading to a increased data log-likelihood.}
    
    \textcolor{gray}{Our multi-modal generative model with latent variable has a fundamental assumption: The conditional distribution of the output variable $\vy$ given the input variable $\vx$, can be related to the latent variable $\vz$, such that $\vy | (\vx, \vz)$ has less uncertainty compared to $\vy | \vx$. Quantitatively, this means $I(\vy;\vz \given \vx) = H(\vz|\vx) - H(\vz|\vy,\vx) = H(\vz) - H(\vz|\vy,\vx) > 0$, where $I(\vy;\vz \given \vx)$ is the mutual information between $\vy$ and $\vz$ conditioned on $\vx$, $H(\vz)$ is the information entropy of $\vz$, and $H(\vz|\vy,\vx)$ is the conditional entropy of $\vz$ conditioned on $\vx$ and $\vy$.}

    \textcolor{gray}{At the beginning of the training of the model, the mutual information $I(\vy;\vz \given \vx)$ is zero because the model has no knowledge of the data, and no corresponding structure has been established in the latent space yet. Along the training, the mutual information increases. For Gaussian posterior $p(\vz \given \vx, \vy)$, this directly leads to a lower determinant of the covariance matrix, which further leads to a decrease in $h(\vmu, \mLambda)$, as shown in \Cref{fig:gap-contour}.}
    
    \begin{figure}
        \centering
        \includegraphics[width=0.6\hsize]{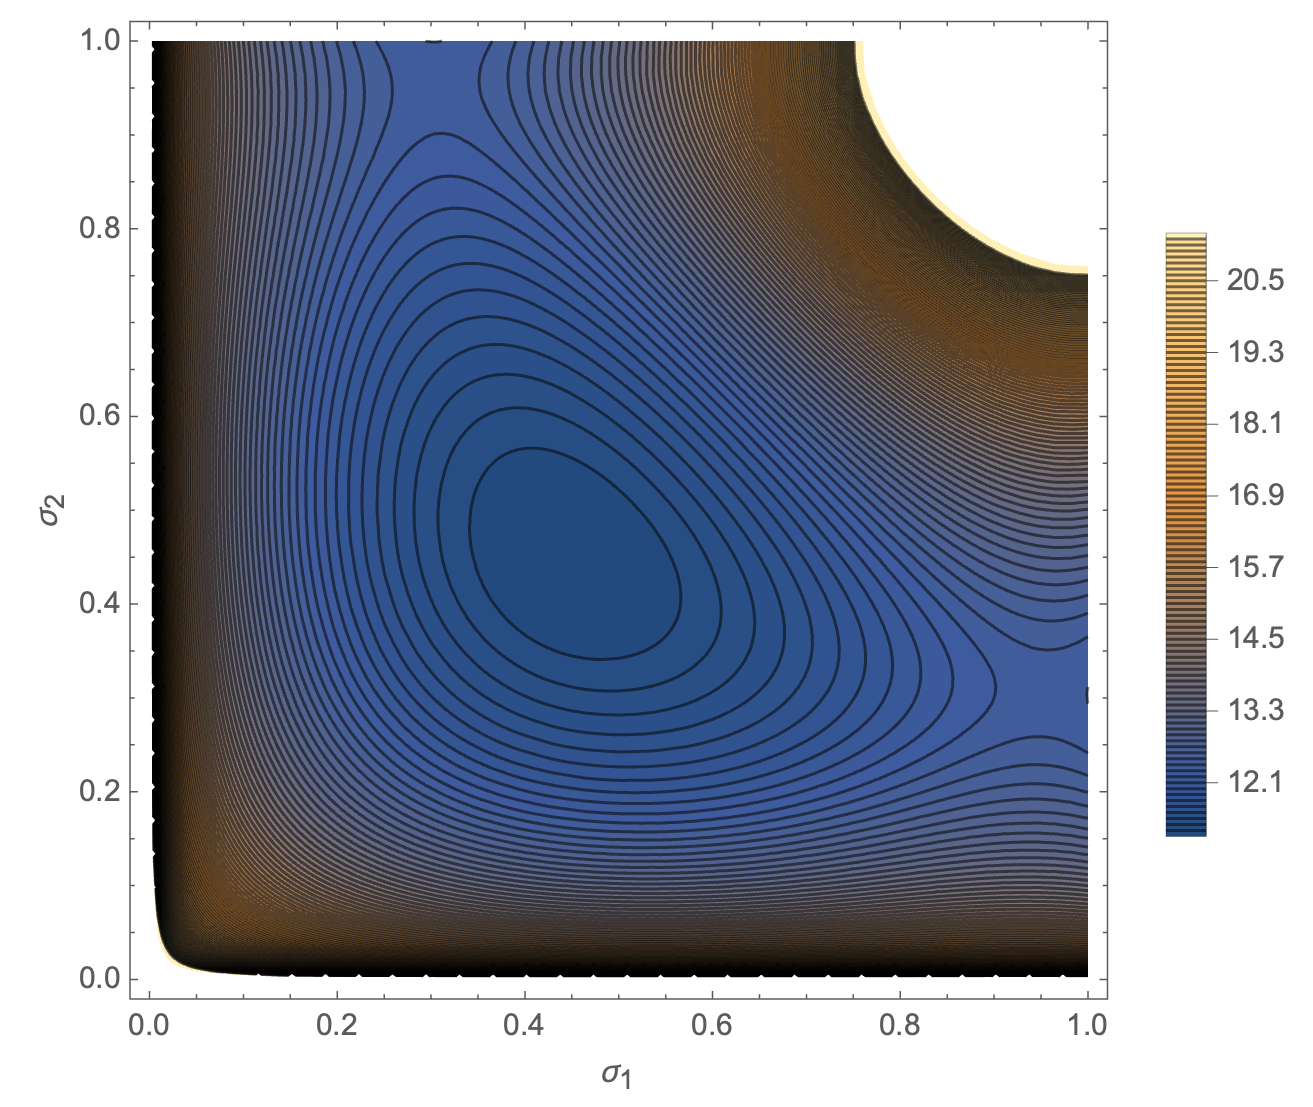}
        \caption{A contour plot demonstration of $h(\vmu, \mLambda)$ for two-dimensional case. The axes correspond to the diagonal elements of $\boldsymbol\Lambda=\text{diag}(\sigma_1^2,\sigma_2^2)$. In this example, $\norm{\vmu}=3.$ }
        \label{fig:gap-contour}
    \end{figure}
    
    \item \textcolor{gray}{The \Cref{fig:gap-contour} shows that the gap becomes large when the posterior variance becomes too small. This happens when the model overfits and a small region in the latent space is over-specialized for certain data, hurting generalization ability.}
    
    \textcolor{gray}{However, such over-specialization can hardly happen in SOG, because the randomized search of the latent code limits the ``resolution'' of the latent code choice and bounds the posterior variance.}% In a $d$-dimensional latent space, if $N$ samples are used for every latent code search, the determinant of posterior variance is effectively bounded below by $1/N$
\end{enumerate}


% One can easily show that $\boldsymbol\mu^T(\mI-\boldsymbol\Sigma)^{-1}\boldsymbol\mu=\Tr(\boldsymbol\mu \boldsymbol\mu^T (\mI-\boldsymbol\Sigma)^{-1}) \leq \|\boldsymbol\mu\|^2 \sqrt{\Tr((\mI-\boldsymbol\Sigma)^{-2})}.$ This uses the inequality that if $A$ and $B$ are positive semidefinite matrices, then $\Tr(AB) \leq \sqrt{\Tr(A^2)\Tr(B^2)}$.
%     Now using the spectral decomposition of the covariance matrix, \begin{subequations}
%     \begin{align}
%         \boldsymbol\mu^T(\mI-\boldsymbol\Sigma)^{-1}\boldsymbol\mu&=\Tr(\boldsymbol\mu \boldsymbol\mu^T (\mI-\boldsymbol\Sigma)^{-1}) \\
%         &\leq \|\boldsymbol\mu\|^2 \sqrt{\Tr((\mI-\boldsymbol\Sigma)^{-2})}.$
%     \end{align}
%     \end{subequations} we get $g(\boldsymbol\mu, \boldsymbol\Sigma) \leq \frac{1}{2}(c \sqrt{\Tr((I- \boldsymbol\Lambda)^{-2})}-\log\det\boldsymbol\Lambda)= h(\boldsymbol\Lambda)$. Recall that $\boldsymbol\Lambda \leq \mI$ and with training the elements of $\boldsymbol\Lambda$ decrease as the posterior gets sharper. Then one can show that $h(\boldsymbol\Lambda)$ decreases initially with training when the the elements of $\boldsymbol\Lambda$ are not too small. Thus, going back to \Cref{eq:BMI} we get that  (data log-likelihood) $\geq$ -(SOG-loss + $h(\boldsymbol\Lambda)$) and with iterations both terms in this lower bound increases initially until the eigenvalues become too small. Thus the log-likelihood of the  data is increased as training progreses. 
