# Supplementary material for: Diverse Imitation Learning via Self-Organizing Generative Models
Source: arXiv:2205.03484 source file (2022-05-06)
Supplement: Supplementary file 6 [file em_toy_rebuttal.tex]

\documentclass{article}

\usepackage[margin=1in]{geometry}
\usepackage{amsmath,amssymb}

\usepackage{graphicx}
\usepackage[export]{adjustbox}
\usepackage{wrapfig}
\usepackage[font=small,labelfont=bf]{caption}

\usepackage{subcaption}  % subfigures
\usepackage{cleveref}

\input{../../math_commands}

\newcommand\givenbase[1][]{\:#1\lvert\:}
\let\given\givenbase
\newcommand\sgiven{\:\lvert\:}

\begin{document}
We further investigate the convergence and final performance of SOG and EM algorithm for the toy example in Appendix A.2.

In Figure 7, the training curves of the two algorithms are plotted in both linear and logarithm scale, and they show that SOG not only has a faster convergence speed, but also a lower loss at convergence, while the posterior distribution of the EM algorithm goes to one-hot just like the hard-assignment used by SOG. This raises the question: now that EM behaves like SOG asymptotically, why does it have inferior performance?

The reason is that, limited by the Gaussian likelihood assumption (which is boundless), EM can never attain purely one-hot posterior, which is shown as follows.

For simplicity, we assume that the three clusters in the toy example are balanced and have the same number of data points. This leads to uniform cluster prior distribution at convergence: $\pi_k^t \rightarrow 1/3, k=1,2,3$. This renders the posterior assignment distribution of a data point over the three clusters simply proportional to the conditional likelihood for the three clusters, i.e.
\[
r_{ik}^{t} = p(z=k \given \vx_i, \vy_i;\: \boldsymbol\theta^{t}, \boldsymbol\Pi^{t}) = \frac{p(\vy_i | \vx_i,z=k;\: \boldsymbol\theta^{t})\:\pi_k^t}{\sum_{l=1}^K p(\vy_i | \vx_i, z=l; \:\boldsymbol\theta^{t})\: \pi_l^t} \approx \frac{p(\vy_i | \vx_i,z=k;\: \boldsymbol\theta^{t})}{\sum_{l=1}^K p(\vy_i | \vx_i, z=l; \:\boldsymbol\theta^{t})} 
\]
Consider a specific data point $(\vx_i, \vy_i)$. Along the training using EM algorithm, one of the cluster, $\kappa$, tends to dominate, so that \[p(\vy_i \given \vx_i, z=\kappa) \gg p(\vy_i \given \vx_i, z=l), \quad \text{if } l \neq \kappa,\]
which is the reason that its posterior distribution tends to one-hot and $r^t_{i\kappa} \approx 1$, while $r^t_{il} \approx 0$ for $l \neq \kappa$.

Now we note that this EM posterior can only finitely approach one-hot when the likelihood function is assumed to be Gaussian, i.e. $p(\vy_i \given \vx_i, z) = \mathcal{N}(\vy; f_\theta(z, \vx), \sigma^2 \mI)$. Because Gaussian likelihood is boundless and is non-zero in the whole domain, and the prediction function $f_\theta$ has finite output, the posterior for the non-dominating clusters is always finite, i.e. $r^t_{il} > 0$ is finite, even for $l \neq \kappa$. This has two consequences:

\begin{enumerate}
    \item The non-dominating clusters will have non-negligible contribution to the loss, not like in SOG. The loss of EM algorithm (we focus on the M-step, because it has direct correspondence to the loss of SOG) for a data point $(\vx_i, \vy_i)$ is given by the expected negative log probability \[\mathcal{L}(\theta) = -\sum_l r^t_{il} \log p(\vy_i \given \vx_i, z=l \;;\; \theta).\] Now that the $r^t_{il}$ is not one-hot, $\log p(\vy_i \given \vx_i, z=l \;;\; \theta)$ will have contribution to the loss for $l\neq \kappa$, making it larger than the loss attained by SOG, where $r^t_{il} = 0$ for $l \neq \kappa$. This is confirmed by the plot \Cref{fig:em-toy-rebuttal:onehot} in where the loss of EM drops significantly when calculated after converting the posterior to exactly one-hot like in SOG.
    
    \item As a consequence, the contribution to the loss from the non-dominating clusters will keep the convergence point slightly away from the optimal solution that maximizes the dominating conditional likelihood $p(\vy_i \given \vx_i, z=\kappa \;;\; \theta)$.
\end{enumerate}

Both of the consequences can be alleviated by decreasing the standard deviation $\sigma$ assumed in the Gaussian likelihood. Indeed, when we decrease $\sigma$ by two orders of magnitude from its original value $1$ to $0.01$, the training curve of EM and SOG match as shown in \Cref{fig:em-toy-rebuttal:low-sigma}.

% This means that $\sigma$ can be used to control the balance between mode specialization and generalization.

\begin{figure}
    \centering
    \begin{subfigure}[t]{0.32\textwidth}
        \centering
        \includegraphics[height=1.8in]{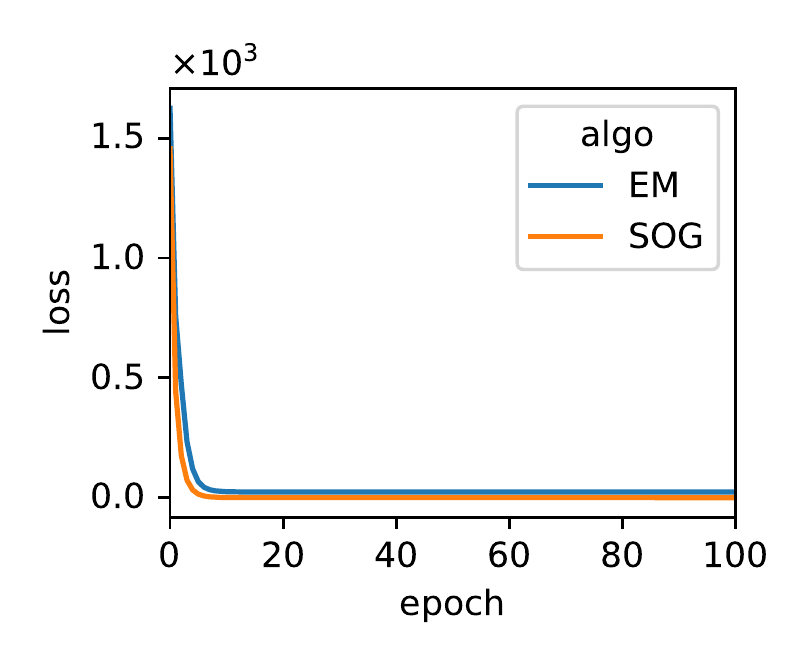}
        \includegraphics[height=1.8in]{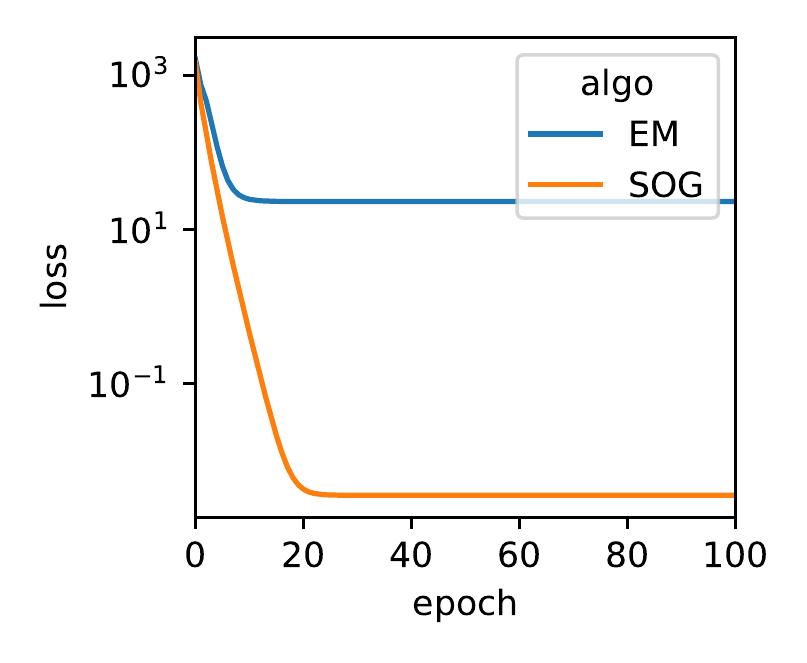}
        \caption{\label{fig:em-toy-rebuttal:original}$\sigma = 1$ for EM. Upper: linear-scale; lower: log-scale}
    \end{subfigure}
    % \hspace{1in}
    \hfill
    \begin{subfigure}[t]{0.32\textwidth}
        \centering
        \includegraphics[height=1.8in]{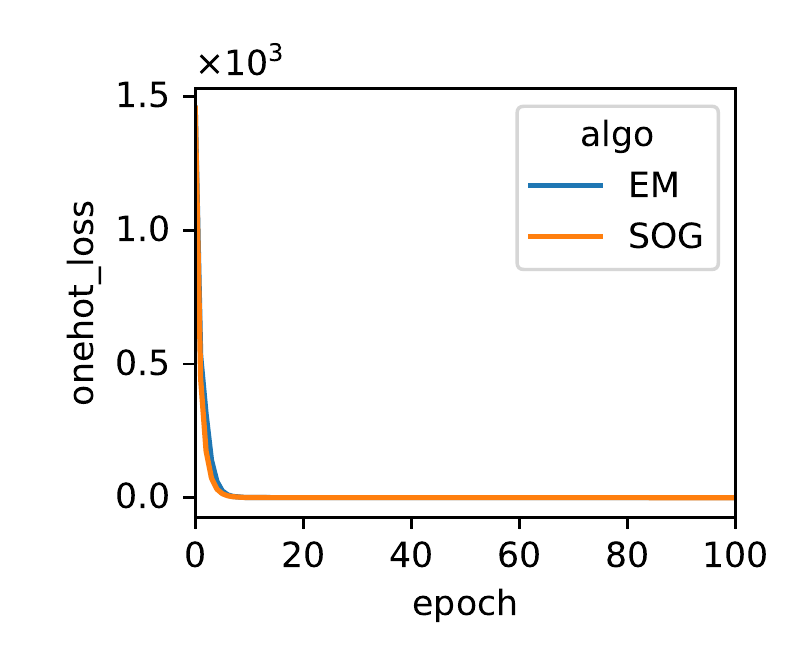}
        \includegraphics[height=1.8in]{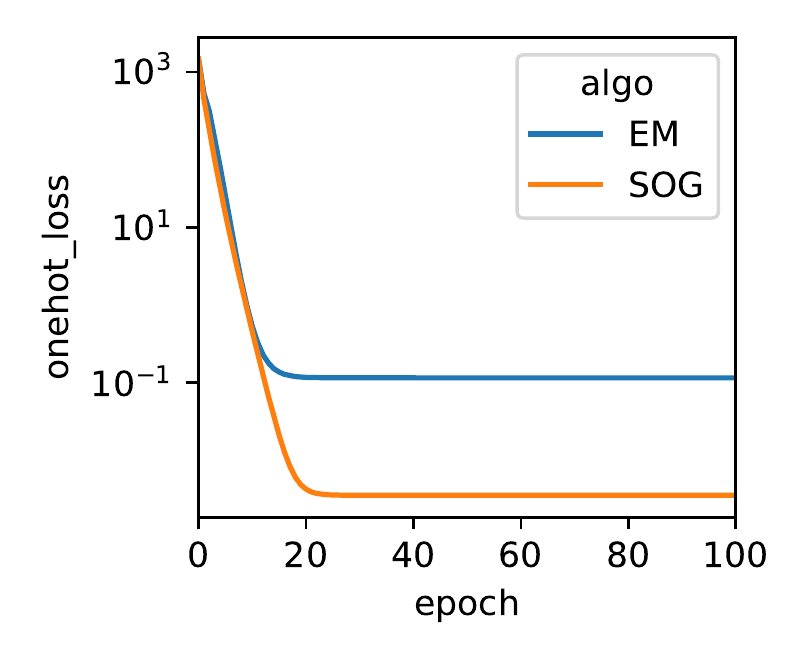}
        \caption{\label{fig:em-toy-rebuttal:onehot}$\sigma = 1$ for EM. Posterior is converted to one-hot when calculating the loss for plotting. Upper: linear-scale; lower: log-scale}
    \end{subfigure}
    \hfill
    \begin{subfigure}[t]{0.32\textwidth}
        \centering
        \includegraphics[height=1.8in]{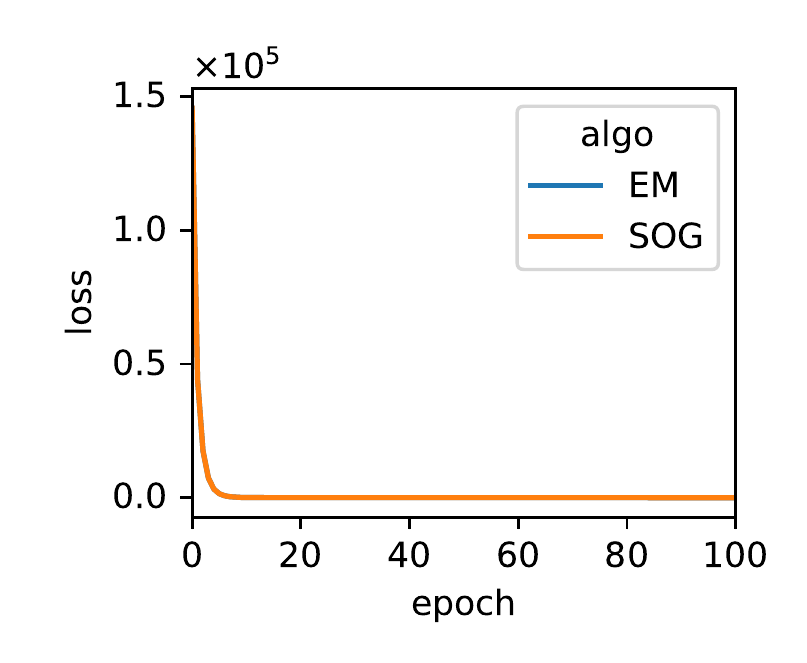}
        \includegraphics[height=1.8in]{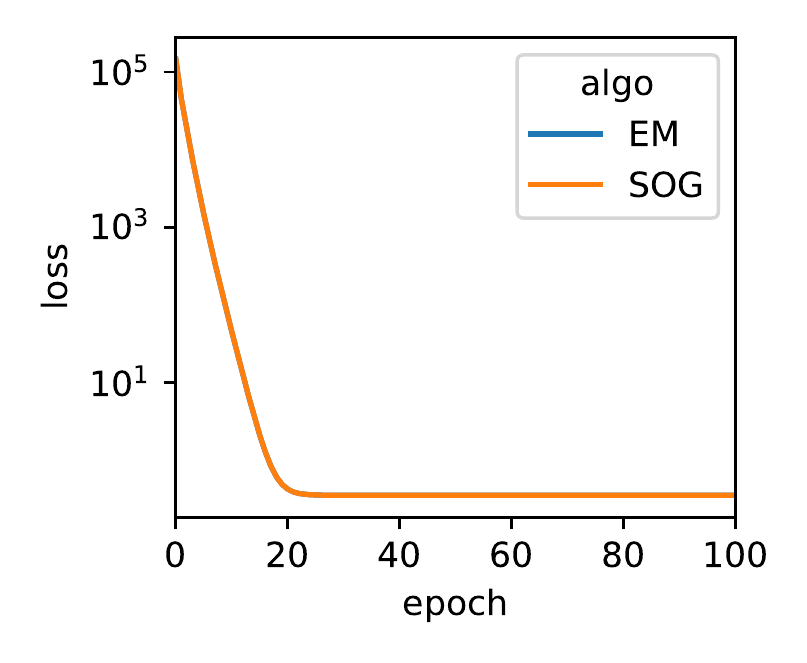}
        \caption{\label{fig:em-toy-rebuttal:low-sigma}$\sigma = 0.01$ for EM. Upper: linear-scale; lower: log-scale}
    \end{subfigure}
    \caption{\label{fig:em-toy-rebuttal} The training curve of the EM algorithm vs that of SOG.}
\end{figure}
\end{document}
